# Supplementary material for: Winding Through: Crowd Navigation via Topological Invariance
Source: arXiv:2109.05084 source file (2022-11-22)
Supplement: Supplementary file 1 [file appendix.tex]

\section*{Appendix}
\renewcommand{\thesubsection}{\Alph{subsection}}\label{sec:appendix}

\subsection{A Deep Reinforcement Learning Oracle}\label{sec:RL}

The performance of our approach relies in the quality of the oracle $\mathcal{O}$ that provides a reference planar trajectory $\tilde{v}_{0:N-1}$. To get a high-quality reference, we employ GA3C-CADRL, the deep reinforcement learning framework of \citet{Everett18_IROS} for multiagent collision avoidance on the plane.

Consider a modified state representation for the robot $\mathrm{s} = \begin{pmatrix} d_g & v_{pref} & \psi & r \end{pmatrix}^{\intercal}$ where $d_g$ is the agent's distance to its goal, $v_{pref}$ is a preferred velocity, and $\psi$ is the robot's orientation\footnote{Since in this work, we do not account for robot orientations, we define $\psi$ to match the direction of the robot's velocity.}, and denote by $\mathrm{s}^i = \begin{pmatrix} x^i & y^i & v^i_x & v^i_y & r^i & d_i & r^i + r \end{pmatrix}^{\intercal}$ the state of agent $i$, where $d_i$ is the distance to the agent's goal. Collect the joint state of the system into $\mathbf{s} = \mathrm{s}\cup_{i=1:n} \mathrm{s}^i$ and define by $\mathrm{u} = (v, \psi)$ the robot's action space. CADRL produces a policy of the form $\pi:\mathbf{s}\to\mathrm{u}$ that maps the joint state of the world to a robot action. 



Considering a reward function of the form
\begin{equation}
R_{col}(\mathbf{s}) =
    \begin{cases}
    1, & \textnormal{if}\: s = s_T\\
    -0.25, & \textnormal{if}\: d_{min} \leq 0\\
    -0.1 + 0.05\cdot d_{min} & \textnormal{if}\: 0 \leq d_{min} \leq 0.2\\
    0, & \textnormal{otherwise}\mbox{,}
    \end{cases}
\end{equation}
where $d_{min}$ is the distance from the robot to the closest agent, GA3C-CADRL recovers an optimal policy $\pi^*(\mathbf{s}) = \arg\min_{\pi} f_{\pi}$ where $f_{\pi}$ is a loss function defined as
\begin{equation}
    f_{\pi} = \log\pi(\mathrm{u}_t|\mathbf{s}_t)(R_t - V(\mathbf{s})) +\beta H(\pi(\mathbf{s}))\mbox{,}
\end{equation}
where 
\begin{equation}
    R_t = \sum_{i = 0}^{k-1}\gamma^i r_{t+i} + \gamma^k V(\mathbf{s})\mbox{,}
\end{equation}
where $V(\mathbf{s})$ is the value function acquired by minimizing in parallel the loss function:
\begin{equation}
    f_v = (R_t - V(\mathbf{s}))^2\mbox{.}
\end{equation}

%employs a deep neural network architecture to jointly learn a policy and value functionapproximate $\pi$ by minimizing 

\subsection{Implementation}

Casadi and other technical details. Share repo? Loop runtime, initialization (seed), everett's implementation


We consider an action space comprising 11 actions in total: 6 actions with fixed speed $v_{pref}$ and heading uniformly sampled from $[-\pi/6,\pi/6]$; 3 actions with fixed speed of $0.5v_{pref}$ and headings $\{-\pi/6, 0, \pi/6\}$; 3 actions with no speed and heading $\{-\pi/6, 0, \pi/6\}$.

\cmnote{how did we tune baselines, TMPC etc}
